# Supplementary material for: RoboVerse: Towards a Unified Platform, Dataset and Benchmark for Scalable and Generalizable Robot Learning
Source: arXiv:2504.18904 source file (2025-04-26)
Supplement: Supplementary file 1 [file contributors.tex]

\section{Contributors and Contribution}

\haoran{will not be included in final paper}

Haoran: Idea proposal, organize team, format design, infra develop, sim transfer
(Isaac Gym, MuJoCo, partial IsaacLab), benchmark transfer (GAPartNet, Open6DOR), Benchmark
Protocol, Policy Training (PoC, DP), Scientific Experiments(Cross sim, sim2real,
sim2sim2real), RL benchmark (propose and help), sim2real (organize team), World
model (data, team), Paper Writing

Feishi: Infra design, Sim transfer (IsaacLab and CoppeliaSim), Format design, Tasks
transfer (RLBench 10/102 to metasim and CALVIN 30/34 to metasim), Policy
Training (Domain randomization implementation), Paper writing

Songlin: Idea discussion, infra implementation, Docker environment setup, task
transfer (GraspNet), Policy Training, Real world Experiments, Paper Writing

Bangjun: Policy data format(RLDS Converter), Benchmark transfer(Isaac Sim:
UniDoorManip, GarmentLab, GAPartNet), Policy Training and \textsc{RoboVerse} Benchmark(PoC,
Baseline implementations: Specialist: ACT, Generalist: Octo, RDT, OpenVLA,
Massive Evaluations), Paper Writing.

Yuran Wang: Diffusion Policy Implementation.

Chengyang Zhao: Diverse demonstration generation for articulated object
manipulation based on GAPartManip. Setup of related tasks in MetaSim.

Jiangran Lyu: Format alignment for rendering(Robocasa), Benchmark transfer(\texttt{robosuite},
Mimicgen), Asset conversion(MJCF to USD)

Jiageng Mao: Implementing Humanoid environment and immigrating UH1 to \textsc{RoboVerse},
support real humanoid robot demos.

Siheng Zhao: Meta-World Benchmark Transfer (Task Config, Asset, Demonstration), Success
Checker, Paper Writing

Chaoyi Xu: teleoperation, rl

Yuxi Qian: Action conditioned Video Generation Model implementation, pretrain +
generation quality experiment on Droid, \textsc{RoboVerse}, droid-roboverse-mix

Charlie Cheng: MuJoCo handler, asset conversion (mjcf2urdf2usd, urdf2mjcf), gapartnet
add trajectory

Peihao Li: LIBERO Benchmark Transfer(config, assets, demo, checker), LIBERO
Benchmark demo scale up, LLM-based Task Generation, MuJoCo handler debug(gripper,
checker)

Yutong Liang: Task migration and RL implementation. Migrate the task of humanoid
robots from HumanoidBench to \textsc{RoboVerse}, especially tasks with rigid and
articulated objects. Improved \textsc{RoboVerse}'s support for MuJoCo, and implemented a
trajectory recorder for humanoid robot. Implemented stable baseline-3 support for
MuJoCo.

Haozhe Chen: Task migration and RL infra implementation. Migrate the tasks, assets and reward functions from HumanoidBench to \textsc{RoboVerse}. Improved \textsc{RoboVerse}'s support for MuJoCo,
and implemented a trajectory recorder for humanoid robot. Implement stable baseline-3 and TDMPC2 support for MuJoCo and IsaacLab.

Haozhe Lou: sim2real experiment for franka and binaul ur5, real2sim code pipeline
in real2sim branch

Mingtong Zhang: gello, sim2real experiment

Boshi: Design and maintain the MetaSim system, adapted 2 simulators (PyBullet, SAPIEN),
transferred RLAfford. Paper writing.

Yufei: Open6DOR data transfer, realistic rendering with Blender, overall writing
refinement
